# Supplementary material for: Self-Supervised Large Scale Point Cloud Completion for Archaeological Site Restoration
Source: arXiv:2503.04030 source file (2025-03-06)
Supplement: Supplementary file 1 [file X_suppl.tex]

\clearpage
\setcounter{page}{1}
\maketitlesupplementary

\setcounter{figure}{0}

\section{General Comparison with Other Methods}

\begin{table*}[!htbp]
    \centering
    \begin{tabular}{|c|c|c|c|c|} % <-- Alignments: 1st column left, 2nd middle and 3rd right, with vertical lines in between
    \hline
      \textbf{Methods} & \textbf{Self Supervised} & \textbf{Spatially imbalanced distribution} & \textbf{Point cloud size} & \textbf{Color} \\
      \hline
      Pcl2Pcl\cite{chen2020pcl2pcl} & \xmark & \xmark & $10k$ & \xmark \\
      PointPnCNet\cite{pointpnc} & \cmark & \xmark & $10k$ & \xmark \\
      P2C\cite{p2c} & \cmark & \xmark & $10k$ & \xmark \\
      ACL-SPC\cite{ACLSPC} & \cmark & \xmark & $10k$ & \xmark \\
      \hline
      Facade\cite{facadeCompletion} & \xmark & \xmark & $>100k$ & \cmark \\
      MCOP \cite{MCOP} & \xmark & \xmark & $>100k$ & \cmark \\
      UAIR \cite{unsupervisedImageInpainting} & \cmark & \xmark & $10k$ & \cmark \\
      SSIM \cite{SSII} & \cmark & \xmark & $10k$ & \cmark \\   
      MCOP + UAIR/SSII & \cmark & \xmark & $>100k$ & \cmark \\
      \hline
      Ours & \cmark & \cmark & $>100k$ & \cmark \\
      \hline
    \end{tabular}
    \caption{Comparison of our method with other SOTA methods in the field of self-supervised point cloud completion. The methods are divided into purely point cloud based ones and view based ones. Our solution works best under the archaeological setting, for example.}
    \label{tab:methodComparisons}
\end{table*}

We list state-of-the-art methods related to our topic (e.g. supervised/unsupervised, point cloud based/view based, etc.) and state  their capability of handling the discussed features under our addressed setting in Tab. \ref{tab:methodComparisons}.

\section{Additional Visualization Results}

\begin{figure*}[!htbp]
\centering
    \begin{minipage}{0.13\linewidth}
    \begin{subfigure}{0.9\linewidth}
    \includegraphics[width=\textwidth]{supplementalImages/site_144_orig.jpg}
    \includegraphics[width=\textwidth]{supplementalImages/site_109_orig.jpg}
    \includegraphics[width=\textwidth]{supplementalImages/site_158_orig.jpg}
    \includegraphics[width=\textwidth]{supplementalImages/site_998_v1_orig.jpg}
    \includegraphics[width=\textwidth]{supplementalImages/site_998_orig_v2.jpg}
    \includegraphics[width=\textwidth]{supplementalImages/site_371_orig_v1.jpg}
    \includegraphics[width=\textwidth]{supplementalImages/site_371_orig_v2.jpg}
    \includegraphics[width=\textwidth]{supplementalImages/site_387_orig.jpg}
    
    \caption{Inputs}
    \end{subfigure}
    % \caption{Figure on right side}\label{fig:right}
    \end{minipage}
    \begin{minipage}{0.13\linewidth}
    \begin{subfigure}{0.9\linewidth}
    \includegraphics[width=\textwidth]{supplementalImages/site_144_p2c.jpg}
    \includegraphics[width=\textwidth]{supplementalImages/site_109_p2c.jpg}
    \includegraphics[width=\textwidth]{supplementalImages/site_158_p2c.jpg}
    \includegraphics[width=\textwidth]{supplementalImages/site_998_p2c_v1.jpg}
    \includegraphics[width=\textwidth]{supplementalImages/site_998_p2c_v2.jpg}
    \includegraphics[width=\textwidth]{supplementalImages/site_371_p2c_v1.jpg}
    \includegraphics[width=\textwidth]{supplementalImages/site_371_p2c_v2.jpg}
    \includegraphics[width=\textwidth]{supplementalImages/site_387_p2c.jpg}

    \caption{P2C}
    \end{subfigure}
    % \caption{Figure on right side}\label{fig:right}
    \end{minipage}
    \begin{minipage}{0.13\linewidth}
    \begin{subfigure}{0.9\linewidth}
    \includegraphics[width=\textwidth]{supplementalImages/site_144_aclspc.jpg}
    \includegraphics[width=\textwidth]{supplementalImages/site_109_aclspc.jpg} 
    \includegraphics[width=\textwidth]{supplementalImages/site_158_aclspc.jpg} 
    \includegraphics[width=\textwidth]{supplementalImages/site_998_v1_aclspc.jpg} 
    \includegraphics[width=\textwidth]{supplementalImages/site_998_aclspc_v2.jpg} 
    \includegraphics[width=\textwidth]{supplementalImages/site_371_aclspc_v1.jpg}
    \includegraphics[width=\textwidth]{supplementalImages/site_371_aclspc_v2.jpg}
    \includegraphics[width=\textwidth]{supplementalImages/site_387_aclspc.jpg}
    
    \caption{ACL-SPC}
    \end{subfigure}
    % \caption{Figure on right side}\label{fig:right}
    \end{minipage}
    \begin{minipage}{0.13\linewidth}
    \begin{subfigure}{0.9\linewidth}
    \includegraphics[width=\textwidth]{supplementalImages/site_144_uair.jpg}
    \includegraphics[width=\textwidth]{supplementalImages/site_109_uair.jpg}
    \includegraphics[width=\textwidth]{supplementalImages/site_158_uair.jpg}
    \includegraphics[width=\textwidth]{supplementalImages/site_998_uair_v1.jpg}
    \includegraphics[width=\textwidth]{supplementalImages/site_998_uair_v2.jpg}
    \includegraphics[width=\textwidth]{supplementalImages/site_371_uair_v1.jpg}
    \includegraphics[width=\textwidth]{supplementalImages/site_371_uair_v2.jpg}
    \includegraphics[width=\textwidth]{supplementalImages/site_387_uair.jpg}

    \caption{UAIR}
    \end{subfigure}
    % \caption{Figure on right side}\label{fig:right}
    \end{minipage}
    \begin{minipage}{0.13\linewidth}
    \begin{subfigure}{0.9\linewidth}
    \includegraphics[width=\textwidth]{supplementalImages/site_144_ssii.jpg}
    \includegraphics[width=\textwidth]{supplementalImages/site_109_ssii.jpg}
    \includegraphics[width=\textwidth]{supplementalImages/site_158_ssii.jpg}
    \includegraphics[width=\textwidth]{supplementalImages/site_998_ssii_v1.jpg}
    \includegraphics[width=\textwidth]{supplementalImages/site_998_ssii_v2.jpg}
    \includegraphics[width=\textwidth]{supplementalImages/site_371_ssii_v1.jpg}
    \includegraphics[width=\textwidth]{supplementalImages/site_371_ssii_v2.jpg}
    \includegraphics[width=\textwidth]{supplementalImages/site_387_ssiiPatch.jpg}

    \caption{SSII}
    \end{subfigure}
    % \caption{Figure on right side}\label{fig:right}
    \end{minipage}
    \begin{minipage}{0.13\linewidth}
    \begin{subfigure}{0.9\linewidth}
    \includegraphics[width=\textwidth]{supplementalImages/site_144_ssiiPatch.jpg}
    \includegraphics[width=\textwidth]{supplementalImages/site_109_ssiiPatch.jpg}
    \includegraphics[width=\textwidth]{supplementalImages/site_158_ssiiPatch.jpg}
    \includegraphics[width=\textwidth]{supplementalImages/site_998_ssiiPatch_v1.jpg}
    \includegraphics[width=\textwidth]{supplementalImages/site_998_ssiiPatch_v2.jpg}
    \includegraphics[width=\textwidth]{supplementalImages/site_371_ssiiPatch_v1.jpg}
    \includegraphics[width=\textwidth]{supplementalImages/site_371_ssiiPatch_v2.jpg}
    \includegraphics[width=\textwidth]{supplementalImages/site_387_ssii.jpg}
    
    \caption{SSII(Patch)}
    \end{subfigure}
    % \caption{Figure on right side}\label{fig:right}
    \end{minipage}
    \begin{minipage}{0.13\linewidth}
    \begin{subfigure}{0.9\linewidth}
    \includegraphics[width=\textwidth]{supplementalImages/site_144_ours.jpg}
    \includegraphics[width=\textwidth]{supplementalImages/site_109_ours.jpg}
    \includegraphics[width=\textwidth]{supplementalImages/site_158_ours.jpg}
    \includegraphics[width=\textwidth]{supplementalImages/site_998_ours_v1.jpg}
    \includegraphics[width=\textwidth]{supplementalImages/site_998_ours_v2.jpg}
    \includegraphics[width=\textwidth]{supplementalImages/site_371_ours_v1.jpg}
    \includegraphics[width=\textwidth]{supplementalImages/site_371_ours_v2.jpg}
    \includegraphics[width=\textwidth]{supplementalImages/site_387_ours.jpg}

    \caption{Ours}
    \end{subfigure}
    % \caption{Figure on right side}\label{fig:right}
    \end{minipage}

  \caption{Additional Visualization of Completion Results of Different Methods.}
  \label{fig:pcdMoreVisualization}
\end{figure*}

In this section we show more visualizations of the completion to walls/structures from archaeological sites not shown in the main text due to limited space. Please see Fig. \ref{fig:pcdMoreVisualization} for more completion results on different types of walls/structures.

\section{Additional Notes on MCOP Images}

We further visualize the details of our enhanced MCOP representation. The scanline trajectory when scanning the structure in the title figure of the main paper is shown in Fig. \ref{fig:scanline zoom in}, which shows the transition from side to top for multiple consecutive slits. 

\begin{figure}[htbp]
    \centering
    \includegraphics[width=0.9\linewidth]{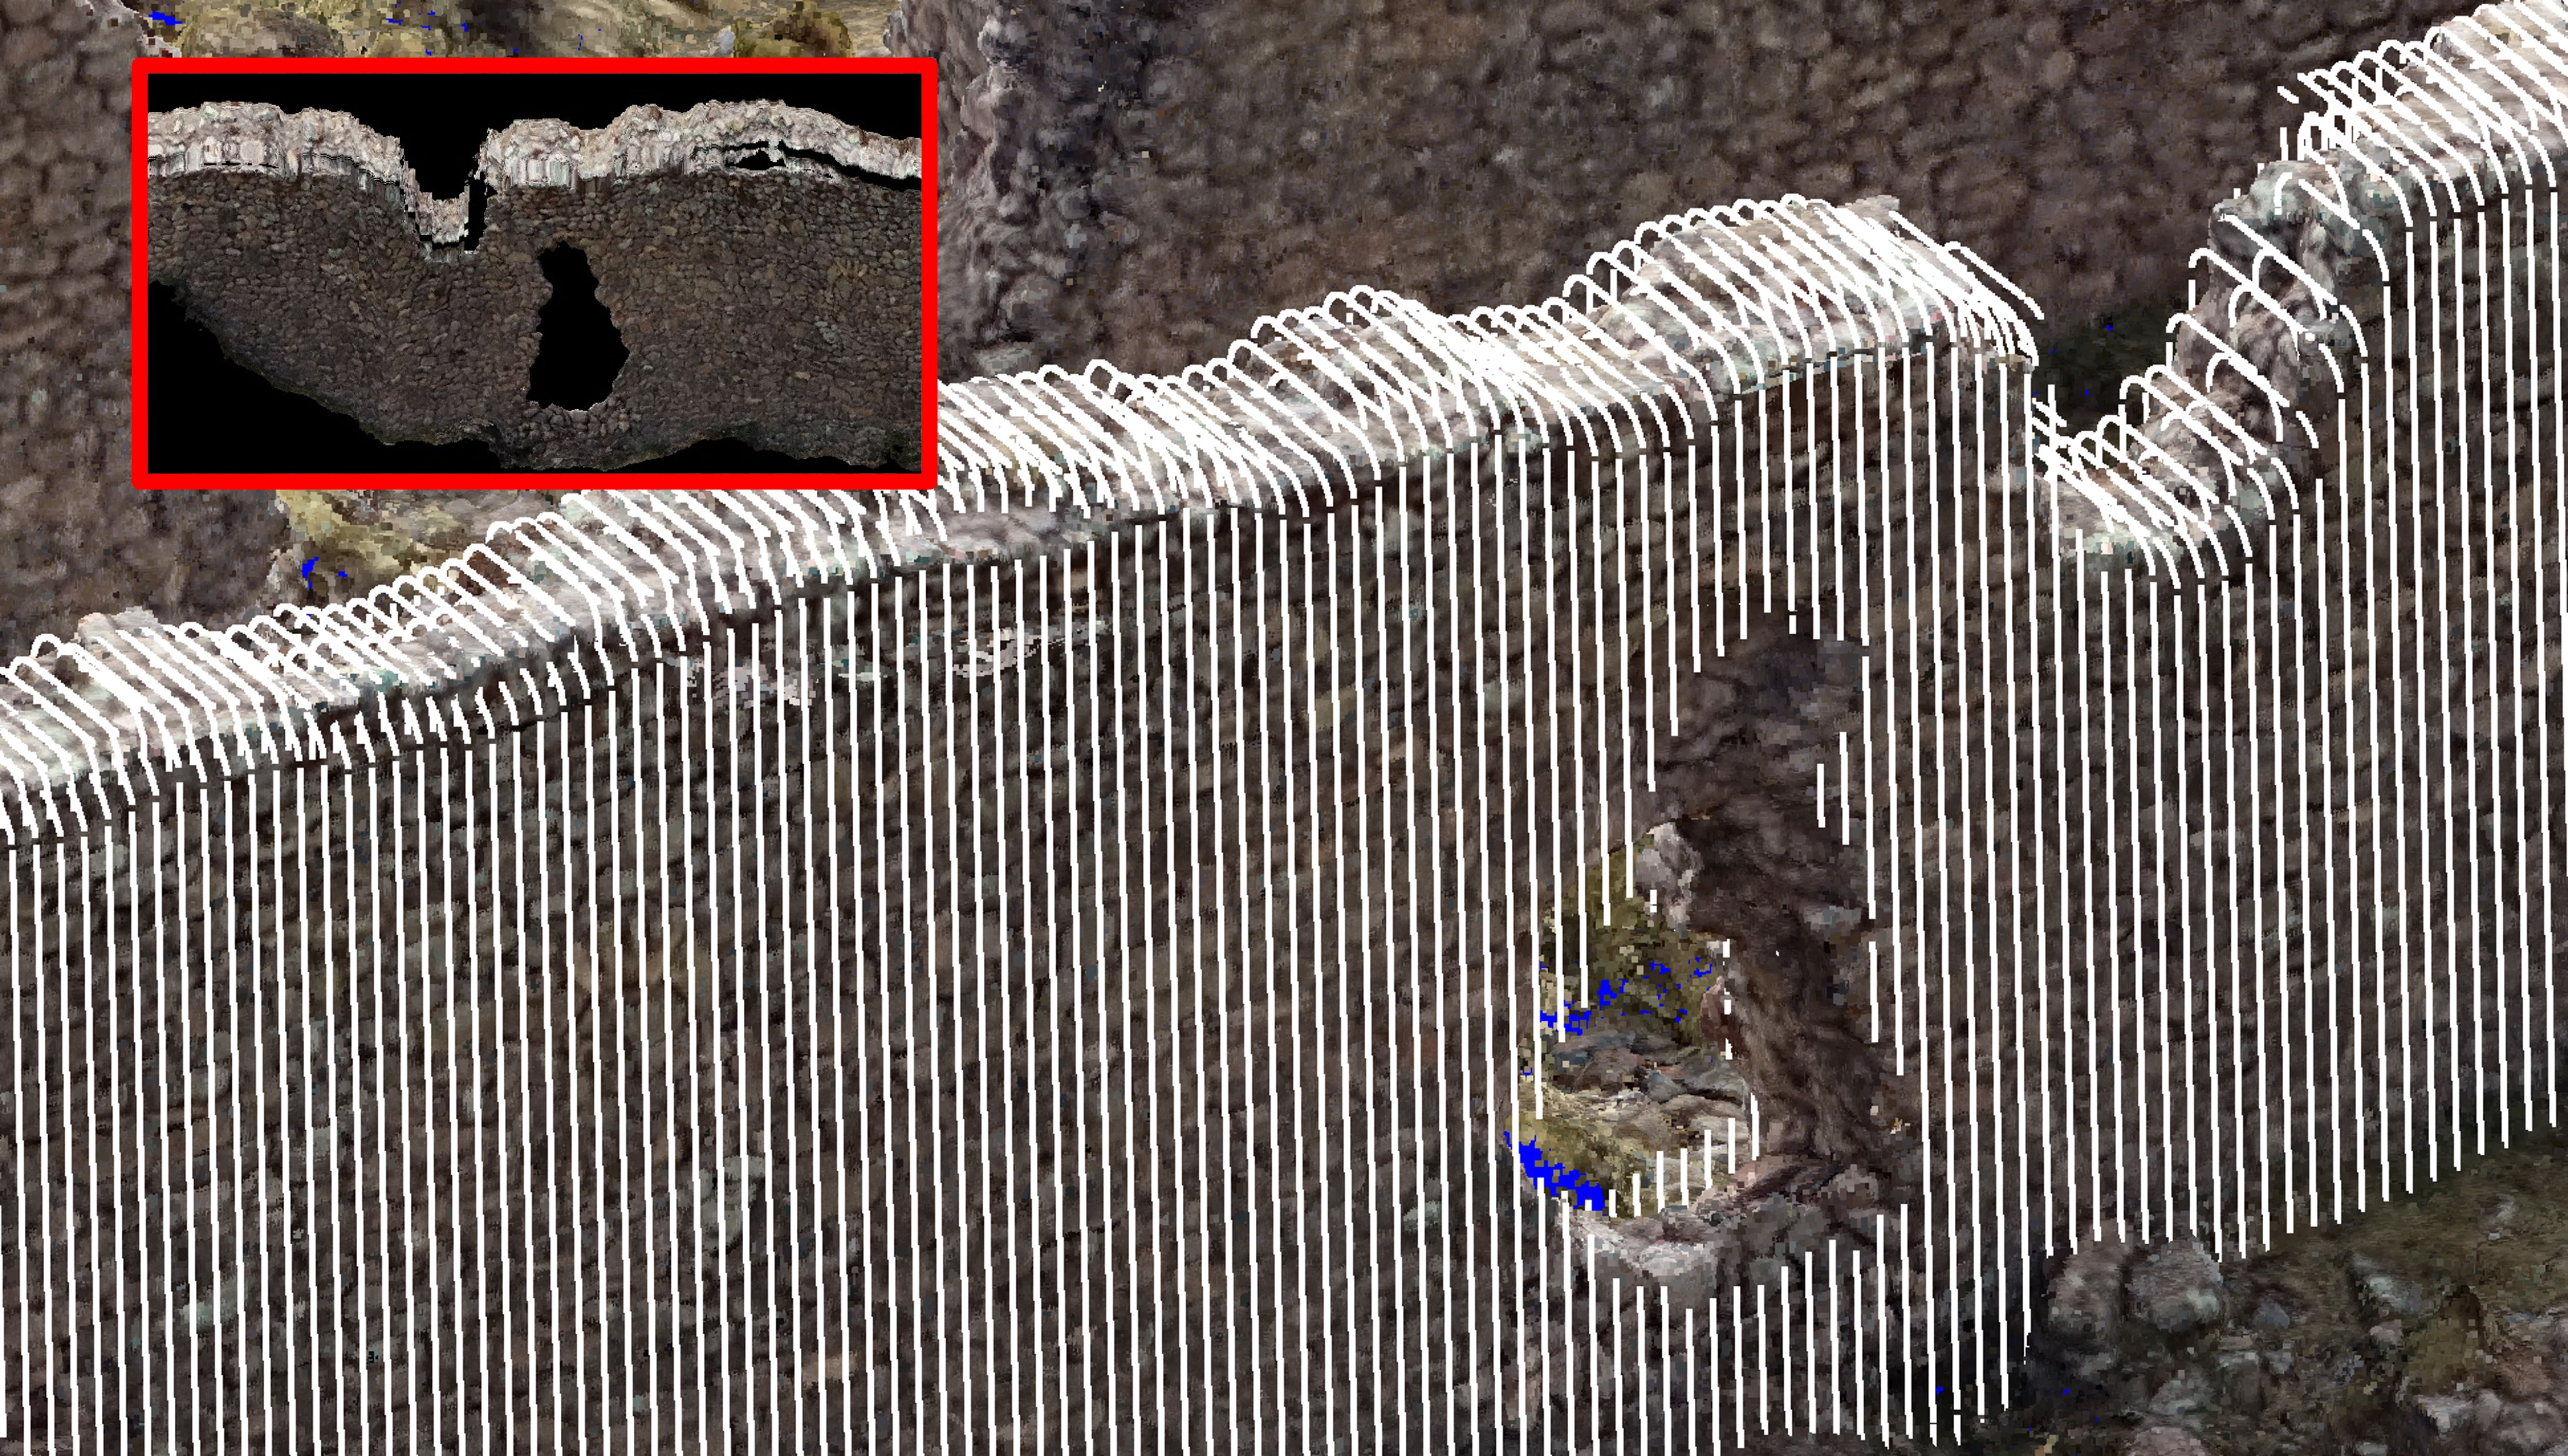}
    \caption{Zoom in view for the structure from the teaser figure in the main paper with the scan line of the camera overlaid. Unlike typical vertical scan trace in \cite{MCOP}, we move the camera smoothly from the side to the top of the target structure, which effectively maintains the geometric locality for points distributed around the transition part.}
    \label{fig:scanline zoom in}
\end{figure}

\begin{figure}[htbp]
    \centering
    \includegraphics[width=\linewidth]{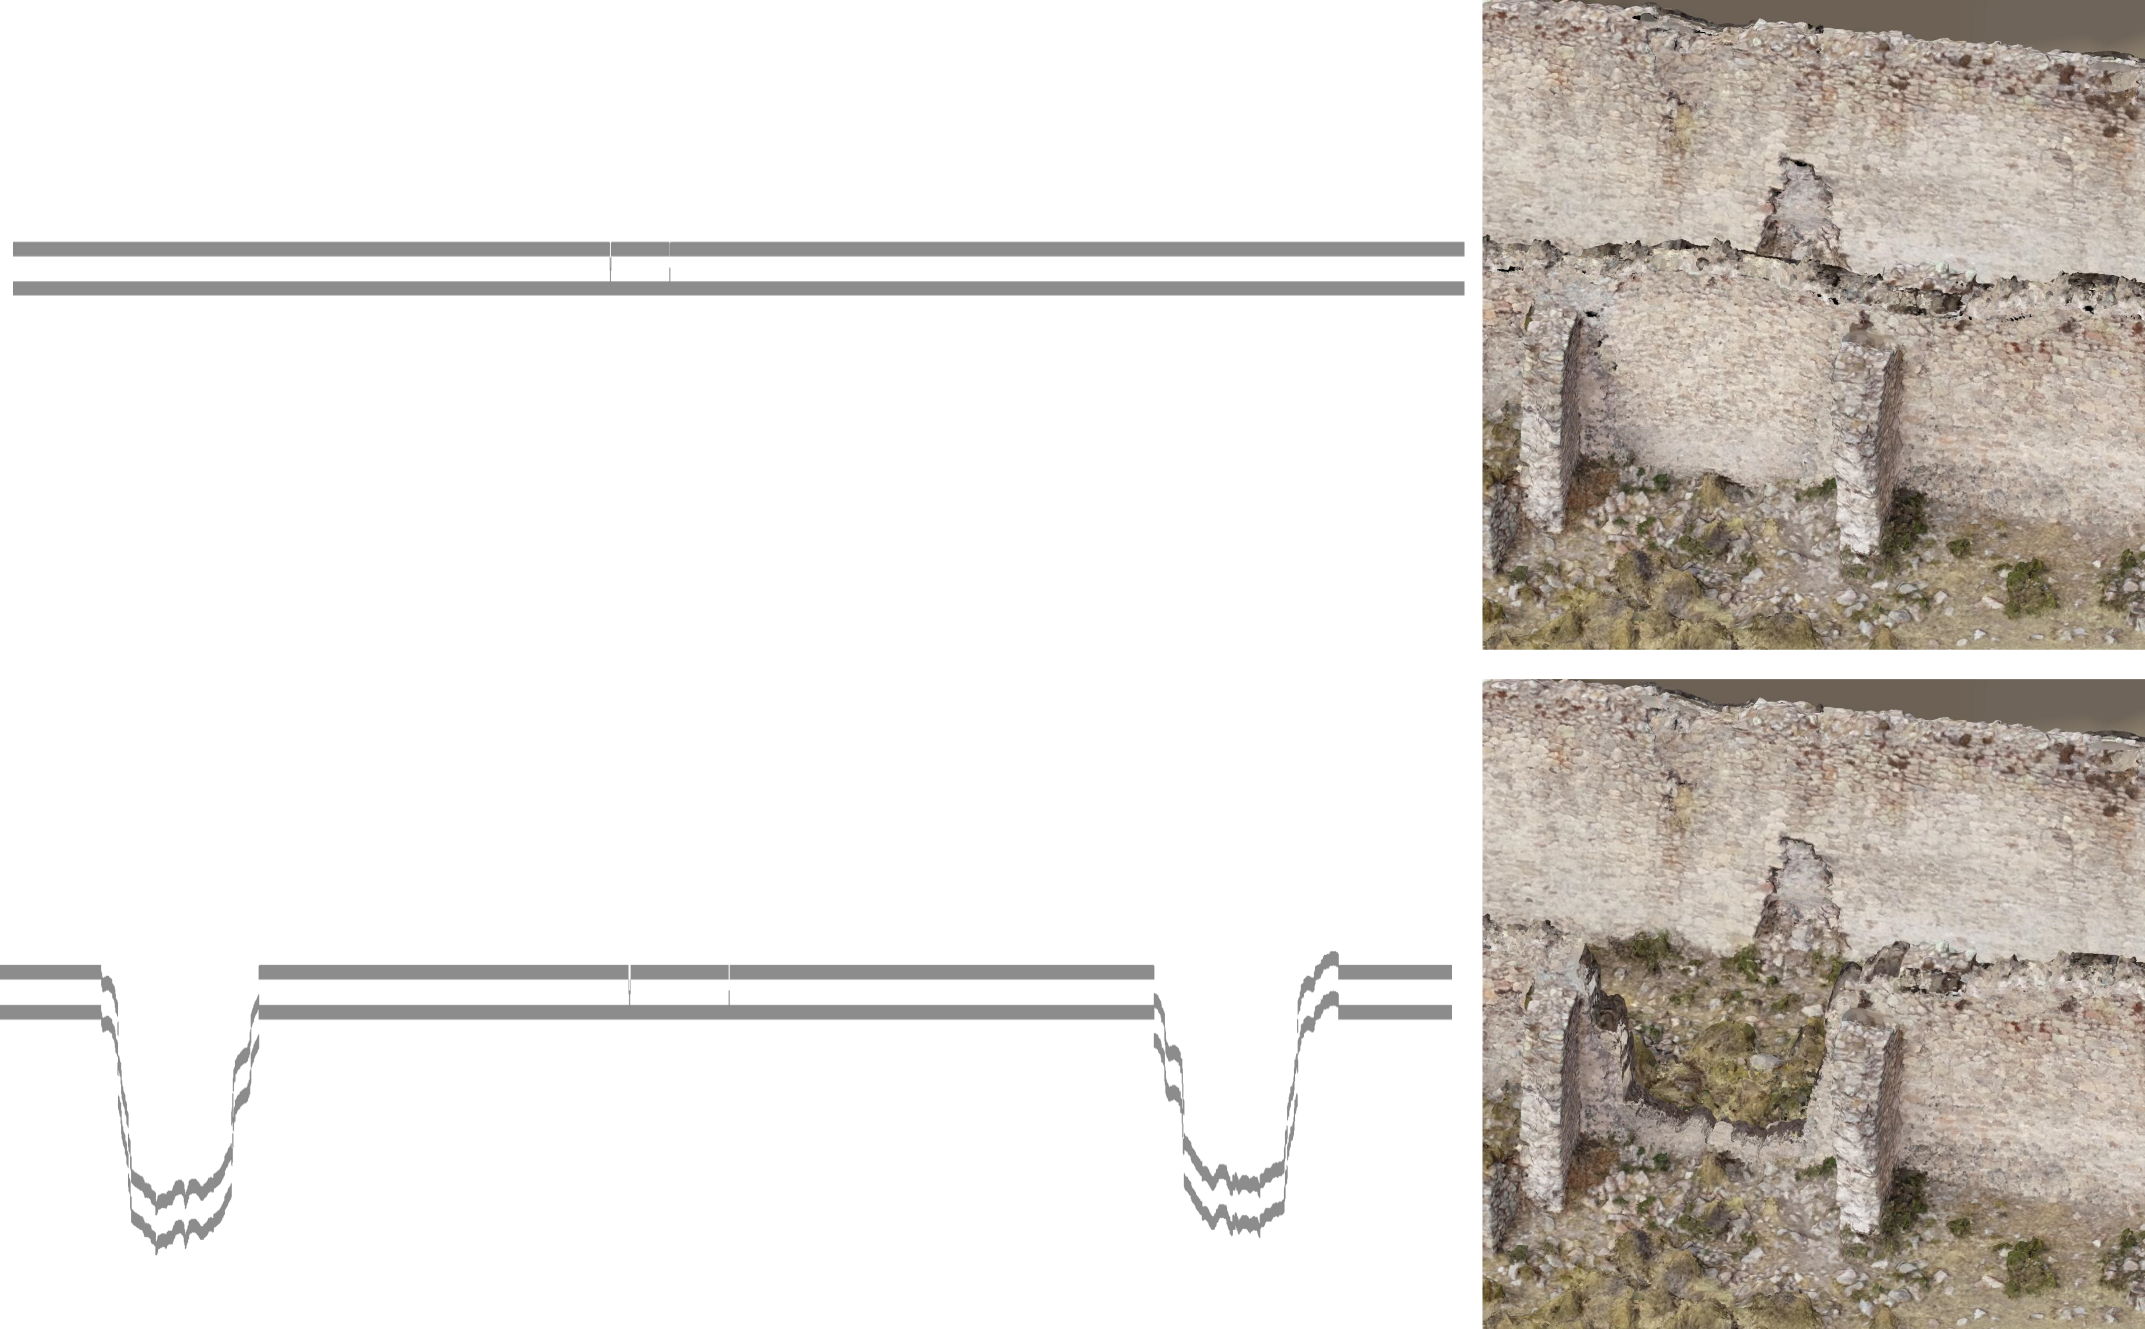}
    \caption{Illustration of how different rotation channels could encode different shape priors for the final completion shape. A uniform rotation map would encourage completion of same height everywhere, while leaving out the necessary boundaries would enable carving out important openings like doors.}
    \label{fig:shape manipulation}
\end{figure}

We also show how the rotation channel enables efficient shape manipulation of the completion. By annotating a rough position of where the slits should turn from side to top (e.g. Fig. \ref{fig:shape manipulation}), we are able to control, for example, whether to complete a door or not in the output point cloud. 

It is noted that the rotation channel annotation does not need to be precisely annotated by the user to receive perfect results. Due to efficient adversarial training on the rotation channel, the completer learns to predict a smooth and genuine looking rotation channel based on the coarse user annotation.

\section{Dataset and training}

\begin{figure}[!htbp]
    \centering
    \includegraphics[width=\linewidth]{supplementalImages/huaDistribution.png}
    \caption{Histogram of random point cloud samples from the Huamanmarca dataset, with high completion ratios at the top to low-completion ratios at the bottom.}
    \label{fig:huamaMissingDistri}
\end{figure}

\begin{figure}[!htbp]
\centering
    \begin{minipage}{0.48\linewidth}
    \begin{subfigure}{0.9\linewidth}
    \includegraphics[width=\textwidth, height=0.5\textwidth]{supplementalImages/color_6_orig.png}
    \includegraphics[width=\textwidth, height=0.5\textwidth]{supplementalImages/color_24_orig.png}
    \includegraphics[width=\textwidth, height=0.5\textwidth]{supplementalImages/color_27.png}
    \includegraphics[width=\textwidth, height=0.5\textwidth]{supplementalImages/color_136_orig.png}
    \caption{Original MCOP images}
    \end{subfigure}
    \end{minipage}
    \begin{minipage}{0.48\linewidth}
    \begin{subfigure}{0.9\linewidth}
    \includegraphics[width=\textwidth, height=0.5\textwidth]{supplementalImages/color_6_adjusted.png}
    \includegraphics[width=\textwidth, height=0.5\textwidth]{supplementalImages/color_24_adjusted.png}
    \includegraphics[width=\textwidth, height=0.5\textwidth]{supplementalImages/color_27_adjusted.png}
    \includegraphics[width=\textwidth, height=0.5\textwidth]{supplementalImages/color_136_adjusted.png}
    \caption{Shadow removed MCOP image}
    \end{subfigure}
    % \caption{Figure on right side}\label{fig:right}
    \end{minipage}

  \caption{Results of manual shadow removal using histogram matching in the preprocessing stage.}
  \label{fig:shadowRemovalIllustration}
\end{figure}

\begin{table}
    \begin{tabular}{l|c|c} % <-- Alignments: 1st column left, 2nd middle and 3rd right, with vertical lines in between
    \hline
      \textbf{Stats} & \textbf{Mawchu} & \textbf{Huaman} \\
      \hline
      \# of structures & 483 & 141 \\
      \hline
      Min size & 0.74k & 485k \\
      Max size & 15 m & 11m \\
      Mean size & 712 k & 1.6m \\ 
      \hline
      Min MCOP size & 0.49 k & 103k \\
      Max MCOP size & 1.9 m & 1.5m  \\
      Mean input MCOP size & 70 k & 575k \\
      \hline
      Min output size & 48 k & 348k  \\
      Max output size & 3.1 m & 4.46m  \\
      Mean output size & 0.31 m & 1.87m \\      
      \hline
      Min missing ratio & 16.8\% & 57.2\% \\
      Max missing ratio & 83.2\% & 76.5\% \\
      Mean missing ratio & 77.0\%  & 68.7\% \\
      \hline
    \end{tabular}
    \caption{Dataset statistics used for qualitative/quantitative evaluation. 
    %The MCOP resolution used in the experiment is determined empirically by decreasing the resolution until observing visible loss of fine details after Poisson Reconstruction.
    }
    \label{table:tmp}
\end{table}

We list a group of important statistics for the evaluation dataset in Table \ref{table:tmp}. As seen, the most important structures consist of nearly millions of points but are still missing many more points. 

The corresponding histogram distribution for completion ratios of structures from \textit{Huamanmarca Raw} is shown in Fig. \ref{fig:huamaMissingDistri}. Unlike \textit{Mawchu Raw} whose structures have completion of varying levels, structures in \textit{Huamanmarca} only have uniformly $20\%$ to $40\%$ available points in the bottom part.

For sites which are reconstructed under illuminance imbalance, we try to recover (or deshadow) with a manual segmentation stage using PhotoShop and separate the relatively dark regions in the MCOP images. The pixels in the dark regions are then transformed using histogram matching with the relatively bright regions within the same structure (e.g. same MCOP image) to maintain better local consistency. A few deshadow results are shown in Fig. \ref{fig:shadowRemovalIllustration}, where the shadow removed structures exhibits better illuminance consistency.
