# Supplementary material for: Self-Supervised Large Scale Point Cloud Completion for Archaeological Site Restoration
Source: arXiv:2503.04030 source file (2025-03-06)
Supplement: Supplementary file 2 [file X_suppl.tex]

\clearpage
\setcounter{page}{1}
\maketitlesupplementary

\section{Rationale}
\label{sec:rationale}
Having the supplementary compiled together with the main paper means that:
\begin{itemize}
\item The supplementary can back-reference sections of the main paper, for example, we can refer to \cref{sec:intro};
\item The main paper can forward reference sub-sections within the supplementary explicitly (e.g. referring to a particular experiment); 
\item When submitted to arXiv, the supplementary will already included at the end of the paper.
\end{itemize}
To split the supplementary pages from the main paper, you can use \href{https://support.apple.com/en-ca/guide/preview/prvw11793/mac#:~:text=Delete%20a%20page%20from%20a,or%20choose%20Edit%20%3E%20Delete).}{Preview (on macOS)}, \href{https://www.adobe.com/acrobat/how-to/delete-pages-from-pdf.html#:~:text=Choose%20%E2%80%9CTools%E2%80%9D%20%3E%20%E2%80%9COrganize,or%20pages%20from%20the%20file.}{Adobe Acrobat} (on all OSs), as well as \href{https://superuser.com/questions/517986/is-it-possible-to-delete-some-pages-of-a-pdf-document}{command line tools}.

\begin{table*}[ht!]
  \begin{center}
    \begin{tabular}{|c|c|c|c|c|} % <-- Alignments: 1st column left, 2nd middle and 3rd right, with vertical lines in between
    \hline
      \textbf{Methods} & \textbf{Self Supervised} & \textbf{Spatially imbalanced distribution} & \textbf{Point cloud size} & \textbf{Color} \\
      \hline
      Pcl2Pcl\cite{chen2020pcl2pcl} & \xmark & ? & $10k$ & \xmark \\
      PointPnCNet\cite{pointpnc} & \cmark & \xmark & $10k$ & \xmark \\
      P2C\cite{p2c} & \cmark & \xmark & $10k$ & \xmark \\
      ACL-SPC\cite{ACLSPC} & \cmark & \xmark & $10k$ & \xmark \\
      MAL-SPC\cite{mal-spc} & \cmark & \xmark & $10k$ & ? \\
      \hline
      Facade\cite{facadeCompletion} & \xmark & \xmark & $>100k$ & \cmark \\
      MCOP \cite{MCOP} & \xmark & \xmark & $>100k$ & \xmark \\
      UAIR \cite{unsupervisedImageInpainting} & \cmark & \xmark & $10k$ & \cmark \\
      MCOP + UAIR + LaMa \cite{LaMa} & \cmark & \xmark & $>100k$ & \cmark \\
      MCOP + UAIR + Latent \cite{latentPaint} & ? & ? & $>100k$ & \cmark \\
      \hline
      Ours & \cmark & \cmark & $>100k$ & \cmark \\
      \hline
    \end{tabular}
        \caption{Comparison of our method with other SOTA methods in the field of self supervised point cloud completion. The methods are divided into purely point cloud based ones and view based ones. Our solution works best under the archaeological setting.}
  \end{center}
\end{table*}

\begin{figure}[htbp]
    \centering
    \includegraphics[width=0.9\linewidth]{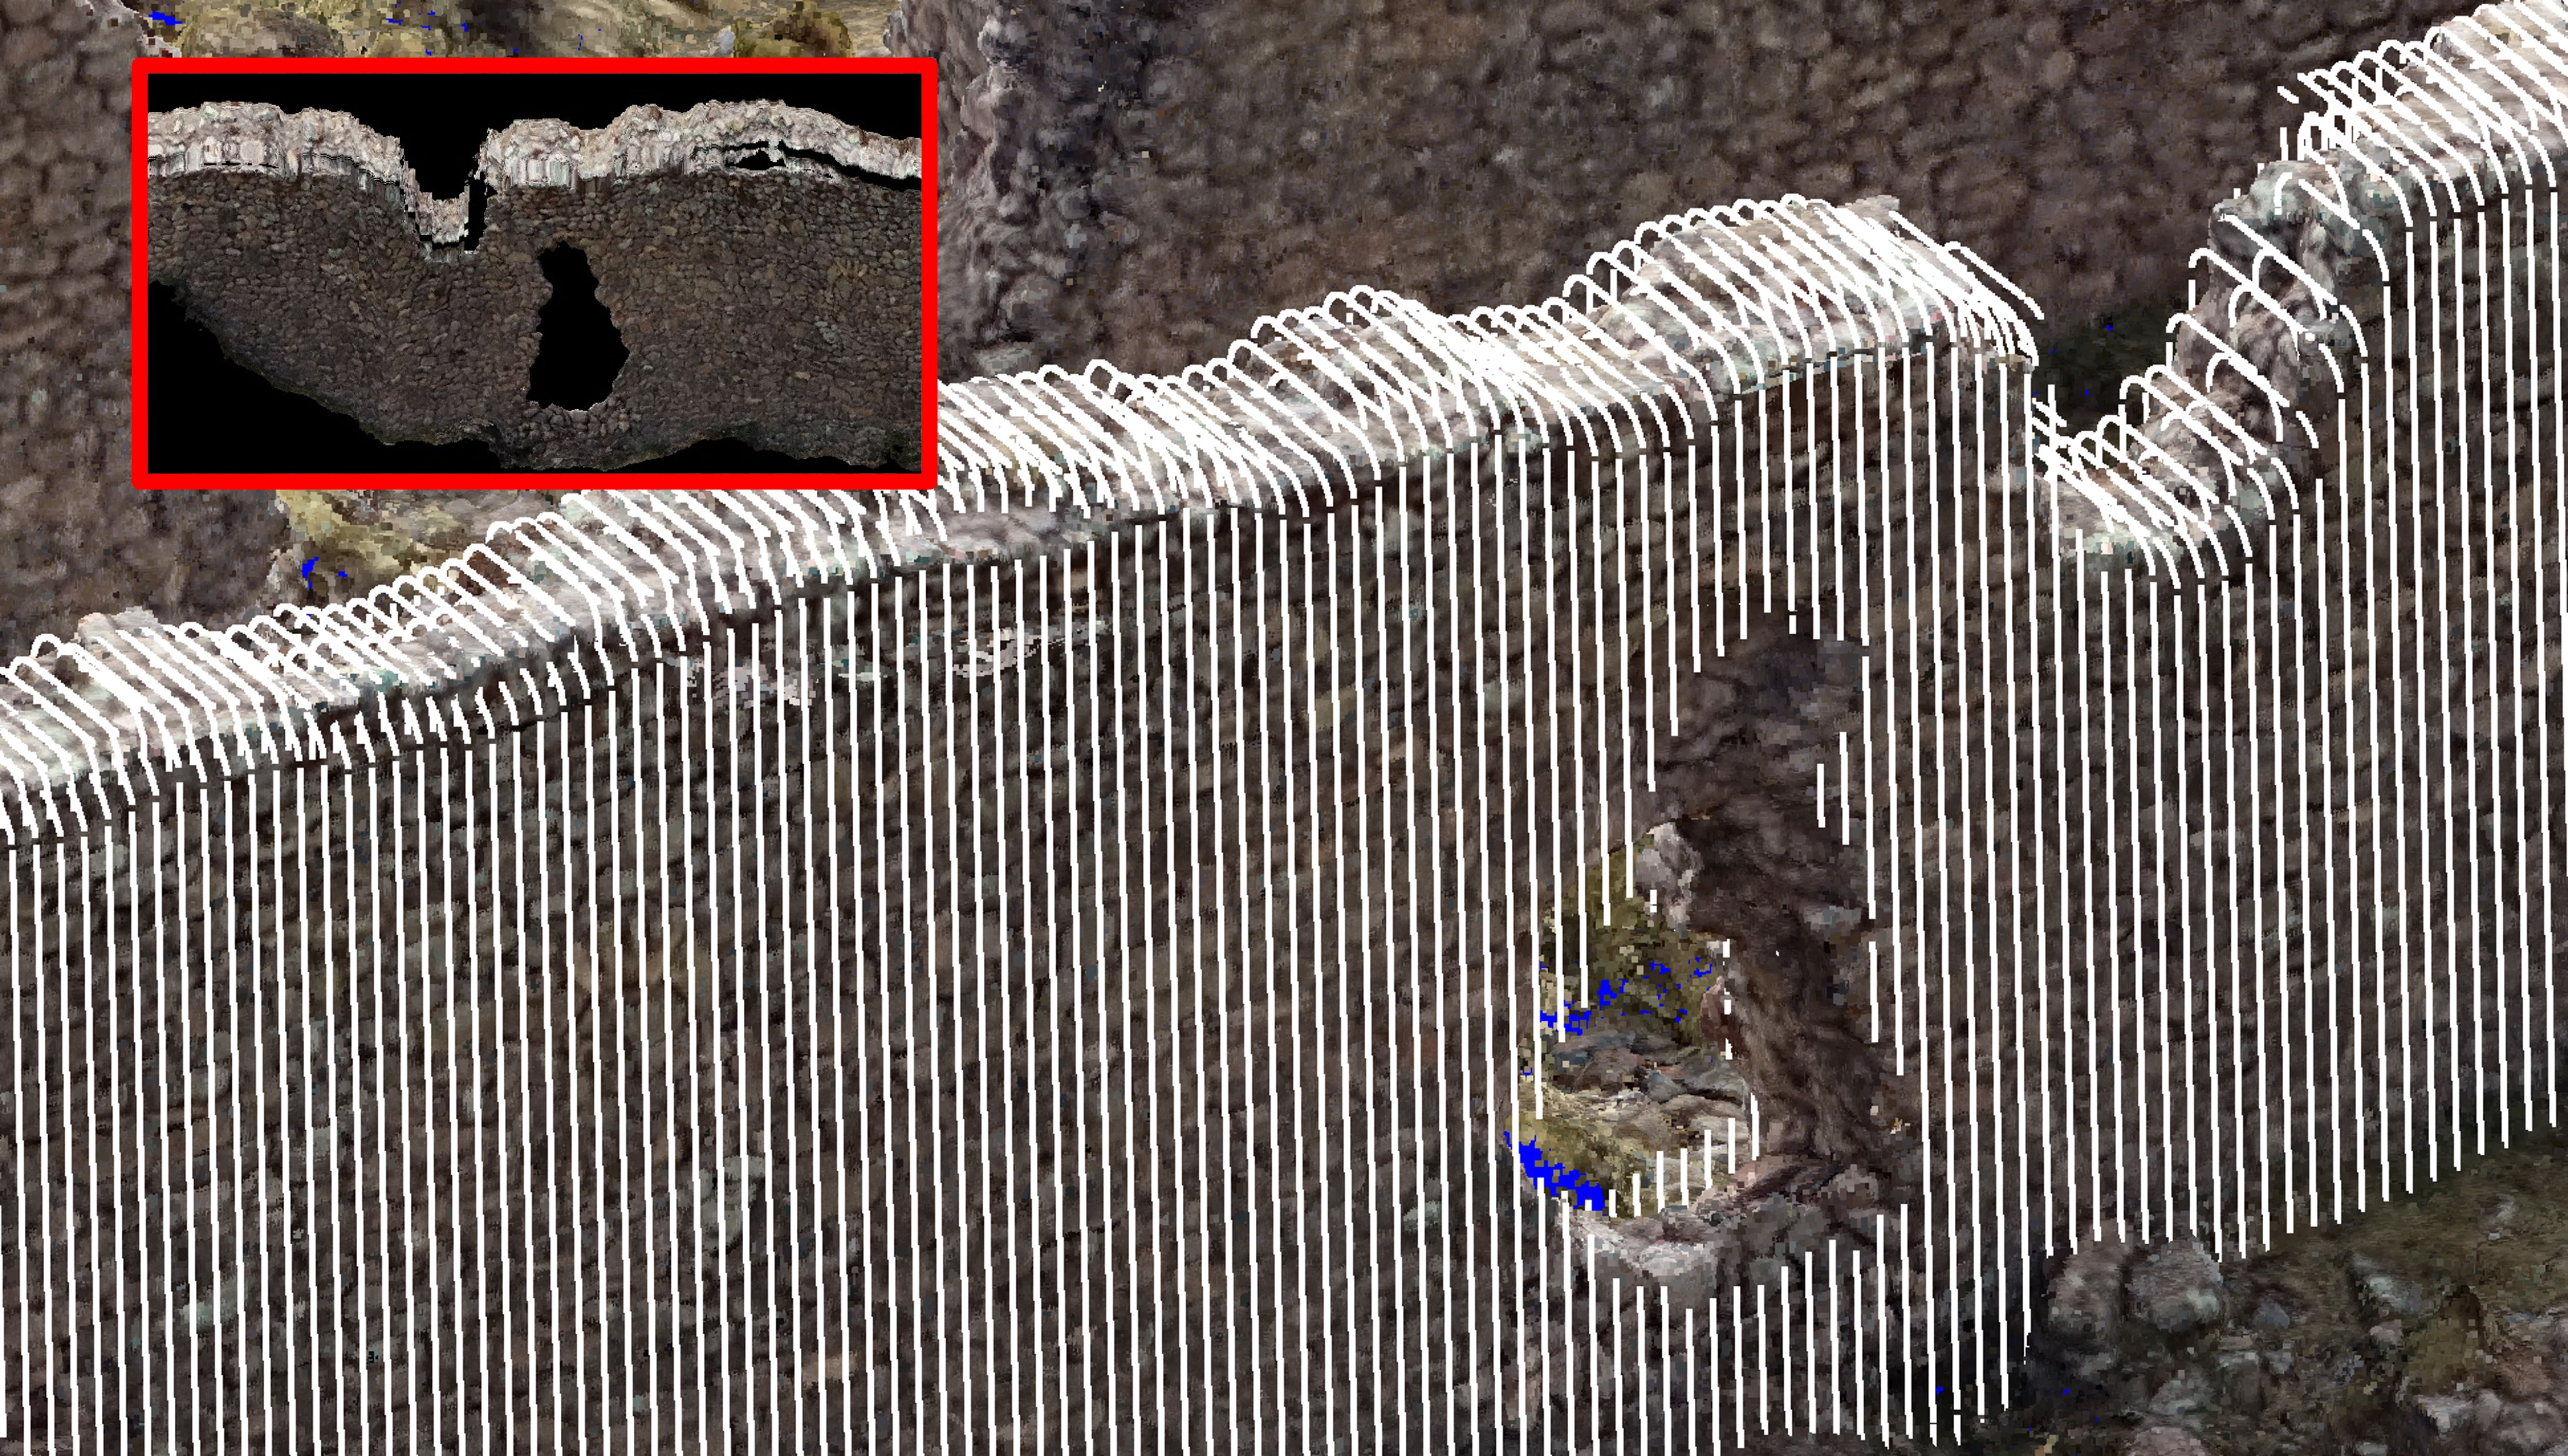}
    \caption{Zoom in view for the structure from Fig. \ref{fig:pipeline} with the scan line of the camera overlaid. Unlike typical vertical scan trace in \cite{MCOP}, we move the camera smoothly from the side to the top of the target structure, which effectively maintains the geometric locality for points distributed around the transition part.}
    \label{fig:scanline zoom in}
\end{figure}

\begin{figure}[htbp]
    \centering
    \includegraphics[width=\linewidth]{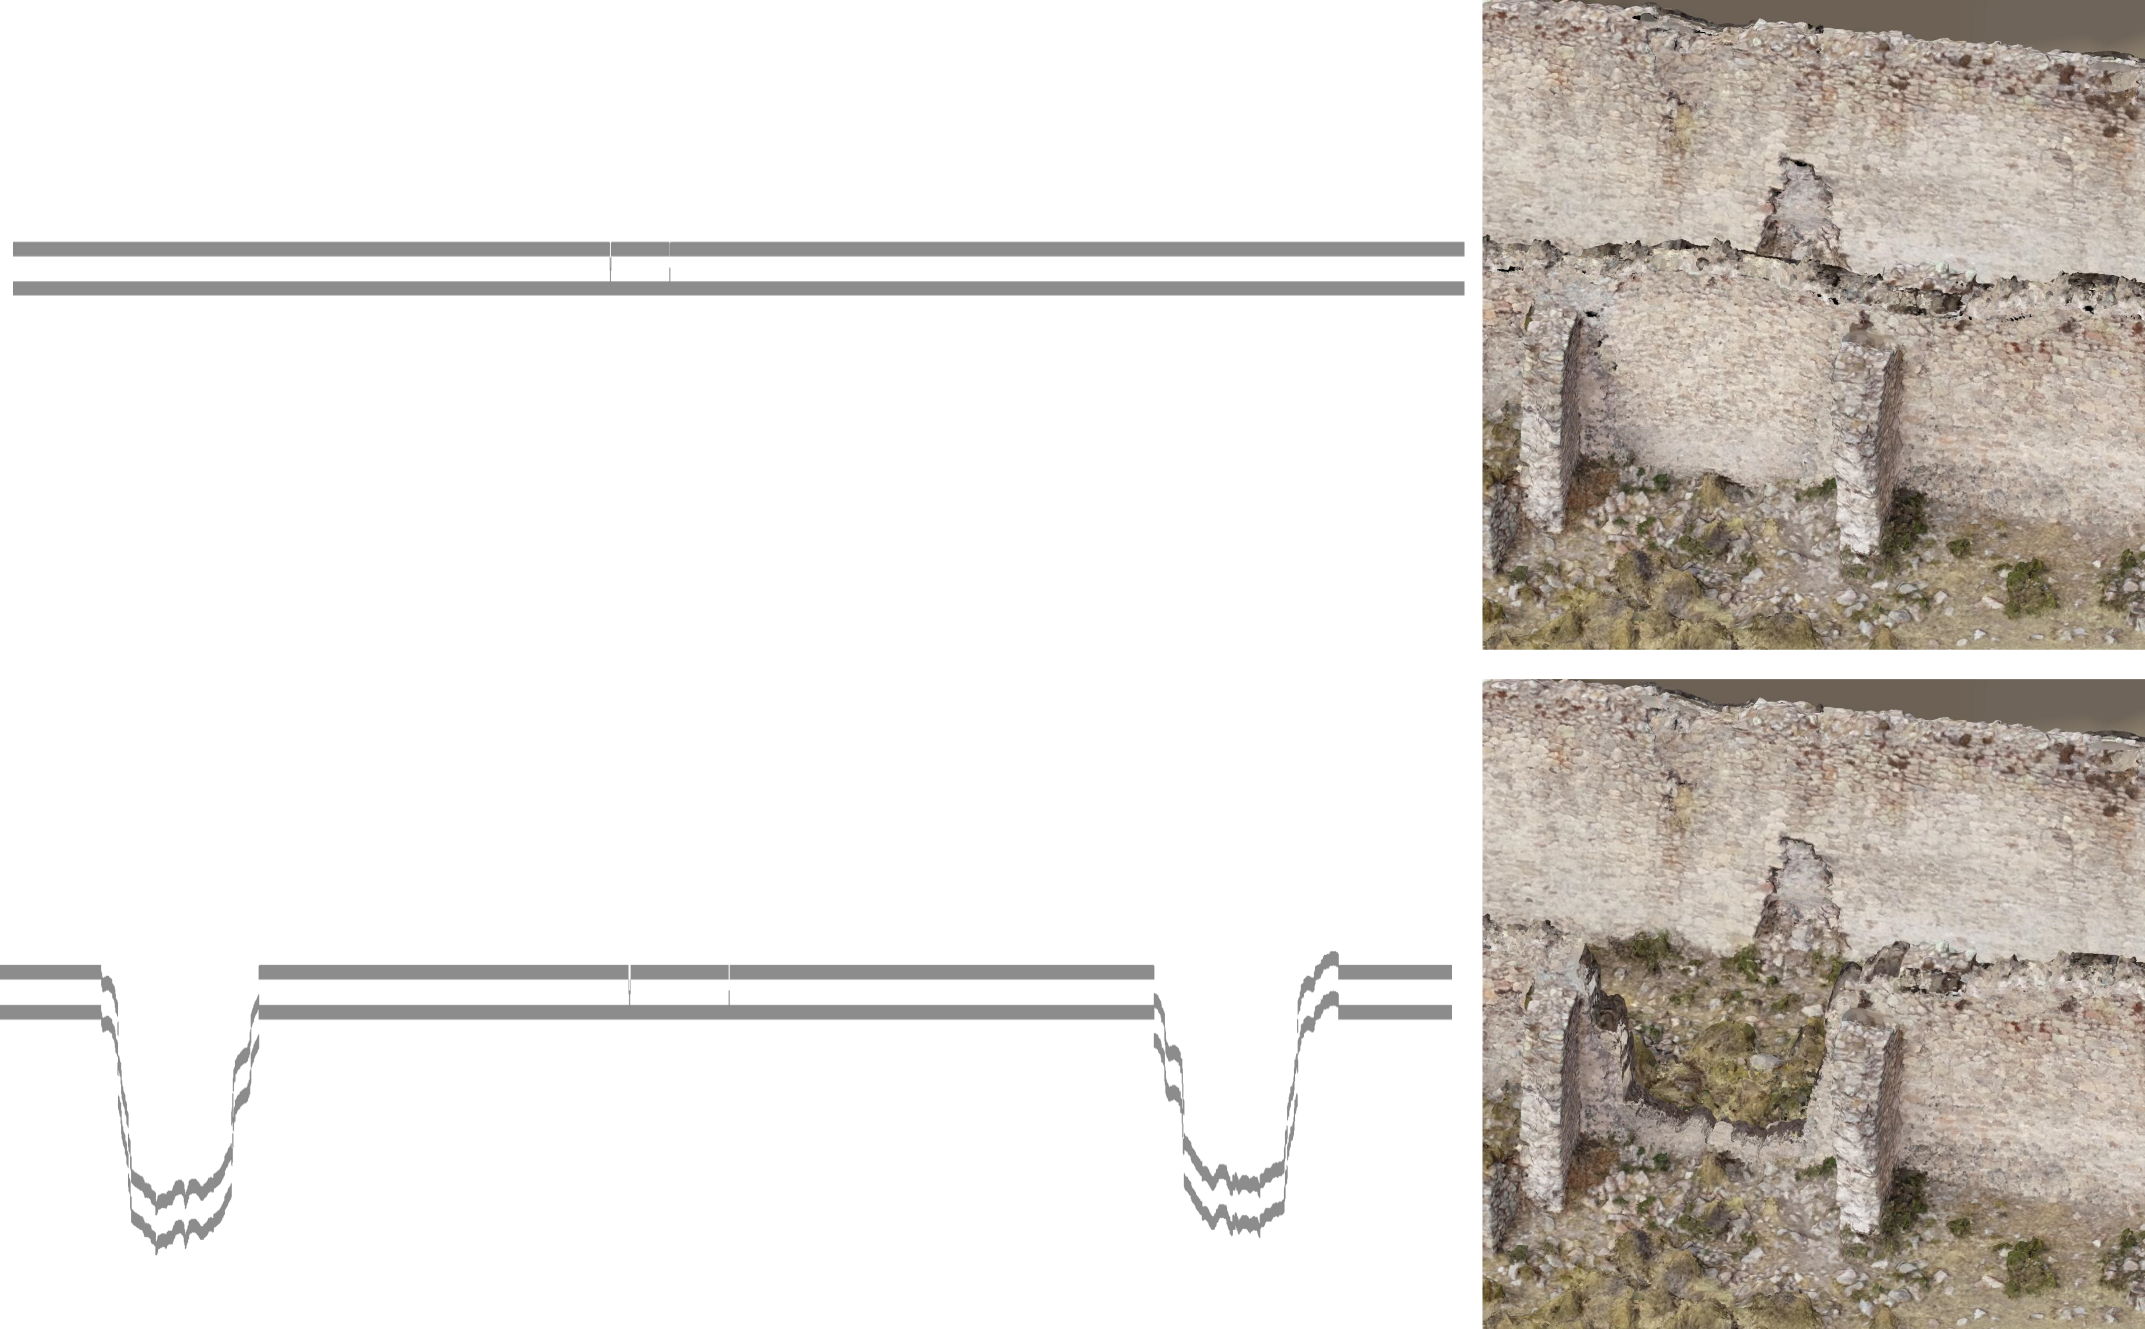}
    \caption{Illustration of how different rotation channels could encode different shape priors for the final completion shape. A uniform rotation map would encourage completion of same height everywhere, while leaving out the necessary boundaries would enable carving out important structures like door.}
    \label{fig:shape manipulation}
\end{figure}

\begin{table}
    \begin{tabular}{l|c|c} % <-- Alignments: 1st column left, 2nd middle and 3rd right, with vertical lines in between
    \hline
      \textbf{Stats} & \textbf{Mawchu} & \textbf{Huaman} \\
      \hline
      \# of structures & 483 & 142 \\
      \hline
      Min size & 0.74k & 485k \\
      Max size & 15 m & 11m \\
      Mean size & 712 k & 1.6m \\ 
      \hline
      Min MCOP size & 0.49 k & 103k \\
      Max MCOP size & 1.9 m & 1.5m  \\
      Mean input MCOP size & 70 k & 575k \\
      \hline
      Min output size & 48 k & 348k  \\
      Max output size & 3.1 m & 4.46m  \\
      Mean output size & 0.31 m & 1.87m \\      
      \hline
      Average missing ratio & 77\%  & 69\% \\
    \end{tabular}
    \caption{Dataset statistics used for qualitative/quantitative evaluation. 
    %The MCOP resolution used in the experiment is determined empirically by decreasing the resolution until observing visible loss of fine details after Poisson Reconstruction.
    }
    \label{table:tmp}
\end{table}
